# Supplementary material for: Active Sampling for Constrained Simulation-based Verification of Uncertain Nonlinear Systems
Source: arXiv:1705.01471 source file (2017-10-01)
Supplement: Supplementary file 1 [file sec_appendix.tex]

\subsection{Batch Active Sampling using Approximate Entropy Reduction}\label{ssec:batchSeq}
Just as with the sequential algorithm in Alg. \ref{alg:sequentialSampling}, the process starts with an initial model and training set $\mathcal{L}$, which is used to compute the entropy (Step 3).  The estimated entropy is then initialized to this quantity.  Steps 4-8 are the main difference between the sequential procedure and this batch process.  Step 5 selects the next sample from the current \textit{estimate} of the entropy, $\hat{H}(\theta|\mathcal{L}\cup\mathcal{S},\sigma)$.  In order to encourage diversity in the points of the batch, this point added to a temporary holding set, $\mathcal{S}$, and removed from $\mathcal{U}$.  Set $\mathcal{S}$ is then used to update the covariance function $\Sigma(\theta)$ to incorporate the effects of the previously selected points in the batch.  The main problem that arises is that the mean function cannot be updated in a similar fashion.  The update of $\mu(\theta)$ would require the measurements $\forall \theta \in \mathcal{S}$, which have not been obtained at that time.  Therefore, the mean is ``held'' at the training set $\mathcal{L}$, defined as $\mu_{\mathcal{L}}(\theta)$, while the covariance is updated with the current $\mathcal{S}$, defined as $\Sigma_{\mathcal{L}\cup\mathcal{S}}(\theta)$.  The updated probability of satisfaction is then approximated using the available information
\begin{equation}\label{eq:approxProb}
	\hat{\mathbb{P}}_+(\theta|\mathcal{L}\cup\mathcal{S},\sigma) = \frac{1}{2}+\frac{1}{2}\text{erf}\bigg(\frac{\mu_{\mathcal{L}}(\theta)}{\sqrt{2\Sigma_{\mathcal{L}\cup\mathcal{S}}(\theta)}}\bigg).
\end{equation}
The approximate probability of satisfaction can then be used to compute the estimated entropy $\hat{H}(\theta|\mathcal{L}\cup\mathcal{S},\sigma)$ in the same manner $\mathbb{P}_{+}(\theta|\mathcal{L},\sigma)$ was used to compute ${H}(\theta|\mathcal{L},\sigma)$ in Eq. \ref{eq:binaryEntropy} (Step 7).  Once a complete batch of $M$ points has been selected, simulations are performed at those locations in $\mathcal{S}$ and the corresponding measurements $y_{\mathcal{S}}$ are taken (Step 9).  Both $\mathcal{S}$ and $y_{\mathcal{S}}$ are added to the training dataset $\mathcal{L}$ and used to retrain the GP model.  Once this has been completed, set $\mathcal{S}$ is emptied and the process is repeated until $T$ iterations are complete.

\begin{algorithm}[H]
\caption{Batch active sampling using approximate entropy reduction}
\label{alg:batchSeq}
\begin{algorithmic}[1]
	\STATE \textbf{Input:} training set $\mathcal{L}$, available sample locations $\mathcal{U}$, trained regression model $\mathcal{GP}$, $T$ batches, $M$ points in each batch, empty set $\mathcal{S}$
	\FOR{$i=1:T$}
	\STATE{Compute entropy $H(\theta|\mathcal{L},\sigma) \ \forall \theta \in \mathcal{U}$, \\set $\hat{H}(\theta|\mathcal{L}\cup\mathcal{S},\sigma) = H(\theta|\mathcal{L},\sigma)$}
	\FOR{$j=1:M$}
	\STATE{Select $\overline{\theta} = \underset{\theta'\in\mathcal{U}}{\text{argmin }} \hat{H}(\theta|\mathcal{L}\cup\mathcal{S},\sigma)$}
	\STATE{$\mathcal{S}$ $\leftarrow$ $\mathcal{S}\cup\overline{\theta}$ and $\mathcal{U}$ $\leftarrow$ $\mathcal{U}\setminus\overline{\theta}$}
	\STATE{Update $\Sigma(\theta)$ with $\theta \in \mathcal{S}$ (but not $\mu(\theta)$) and recompute $\hat{H}(\theta|\mathcal{L}\cup\mathcal{S},\sigma)$}
	\ENDFOR
	\STATE{Run simulations $\forall \theta\in\mathcal{S}$, obtain $y_{\mathcal{S}}$}
	\STATE{$\mathcal{L}$ $\leftarrow$ $\mathcal{L}\cup\{\mathcal{S},y_{\mathcal{S}}\}$}
	\STATE{Reinitialize empty $\mathcal{S}$, retrain $\mathcal{GP}$ with new $\mathcal{L}$}
	\ENDFOR
\end{algorithmic}
\end{algorithm}

\subsection{k-Determinantal Point Processes for Sampling}\label{ssec:kDPP}
Determinantal Point Processes (DPPs) are useful tools for selecting sets of samples where diversity in the samples is important\cite{Kulesza12_FTML}.  In these approaches, a set of samples generated according to the underlying probability distribution is used to construct a DPP, which then can be used to produce a second sample set of the same size with a higher level of diversity.  In many applications, only a small number of samples are desired; however, the DPP loses its utility when it is constructed from a small number of initial samples.  For these problems, k-DPPs\cite{Kulesza11_ICML} were developed to obtain a small set of samples (of size $k$) from a DPP with a larger initial set of samples.  The following algorithm describes k-DPP based sampling as it relates to the simulation-based verification procedure.

The procedure assumes $M_T$ samples of $\theta$ have been generated according to $\mathbb{P}_H(\theta)$ formed from the entropy $H(\theta|\mathcal{L},\sigma)$.  In order to have a suitable number of samples to construct the DPP, $M_T \approx 1000$ for the examples in this paper.  These samples form a matrix $L$ that measures correlation between samples (Step 4).  An isotropic squared exponential kernel is used to measure similarity and ensure the components of $L$ are $L(i,j) \leq 1$ and $L$ is positive definite.  The term $l$ is the lone hyperparameter of the RBF kernel.  This term was set to $l=5$ for the examples.  Next, the eigenvalues $\lambda_j$ and eigenvectors $v_j$ of $L$ are found (Step 7).  The eigenvalues are also used to compute the corresponding elementary symmetric polynomials $e_m$.  These elementary polynomials and the eigenvalues compute the marginal and sampling from marginal in Step 10, adding indices to set $J$.  Once the loop has run out of remaining indices, a sample $y_i$ from the set of all indices is chosen and added to $Y$ in Steps 21 and 22.  The eigenvector corresponding to $y_i$ is then removed from the set $V$ of all remaining eigenvectors.  Steps 21-23 are repeated until $M$ samples have been chosen, completing the batch.  Note that the values in the output set $Y$ correspond to \textit{indices} of $\theta$ terms in the initial input set of $M_T$ $\theta$ values sampled from $\mathbb{P}_H(\theta)$.  The actual sample locations are taken from that set of $M_T$ points.

\begin{algorithm}[H]
\caption{k-DPP sampling algorithm; adapted from\cite{Kulesza11_ICML}.}
\label{alg:kDPP}
\begin{algorithmic}[1]
	\STATE \textbf{Input:} $M_{T}$ randomly generated samples of $\theta$, empty set $J$, $M$ points in batch
	\FOR{$i=1:M_T$}
		\FOR{$j=1:M_T$}
		\STATE{Compute $L(i,j) = e^{-||\theta_i-\theta_j||^2/l^2}$}
		\ENDFOR
	\ENDFOR
	\STATE{Eigendecomposition of $L$ $\rightarrow$ $\{v_j,\lambda_j\}$}
	\STATE{Initialize $m = M$}
	\FOR{$j=M_T:-1:1$}
		\IF{$u \sim \text{Uniform}[0,1] < \lambda_j \frac{e_{m-1}^{j-1}}{e_m^j}$}
		\STATE{$J\leftarrow J\cup\{j\}$}
		\STATE{$m\leftarrow m-1$}
		\IF{$m=0$}
		\STATE \textbf{break}
		\ENDIF
		\ENDIF
	\ENDFOR
	\STATE{$V\leftarrow \{v_j\}j\in J$}
	\STATE{$Y\leftarrow \emptyset$}
	\WHILE{$|V| >0$}
	\STATE{Select $y_i$ with probability $\mathbb{P}(y_i) = \frac{1}{|V|}\sum_{v\in V}(v^T e_i)^2$}
	\STATE{$Y\leftarrow Y\cup y_i$}
	\STATE{$V\leftarrow V_{\perp}$ (orthonormal basis for subspace of $V$ orthogonal to $e_i$)}
	\ENDWHILE
	\STATE \textbf{Output:} sample set $Y$ of size $M$
\end{algorithmic}
\end{algorithm}
